# Supplementary material for: P3: Toward Privacy-Preserving Photo Sharing
Source: arXiv:1302.5062 source file (2013-02-20)
Supplement: Supplementary file 1 [file appendix.tex]

\appendix
\section{The Examined Images}
\label{appx:rawimages}

In this section, we provide a set of images used for the evaluation.
Each raw image is presented with its canny edge detection result.

\begin{figure}
    \centering
    \includegraphics[viewport=0 200 800 550, scale=0.32, clip=true]{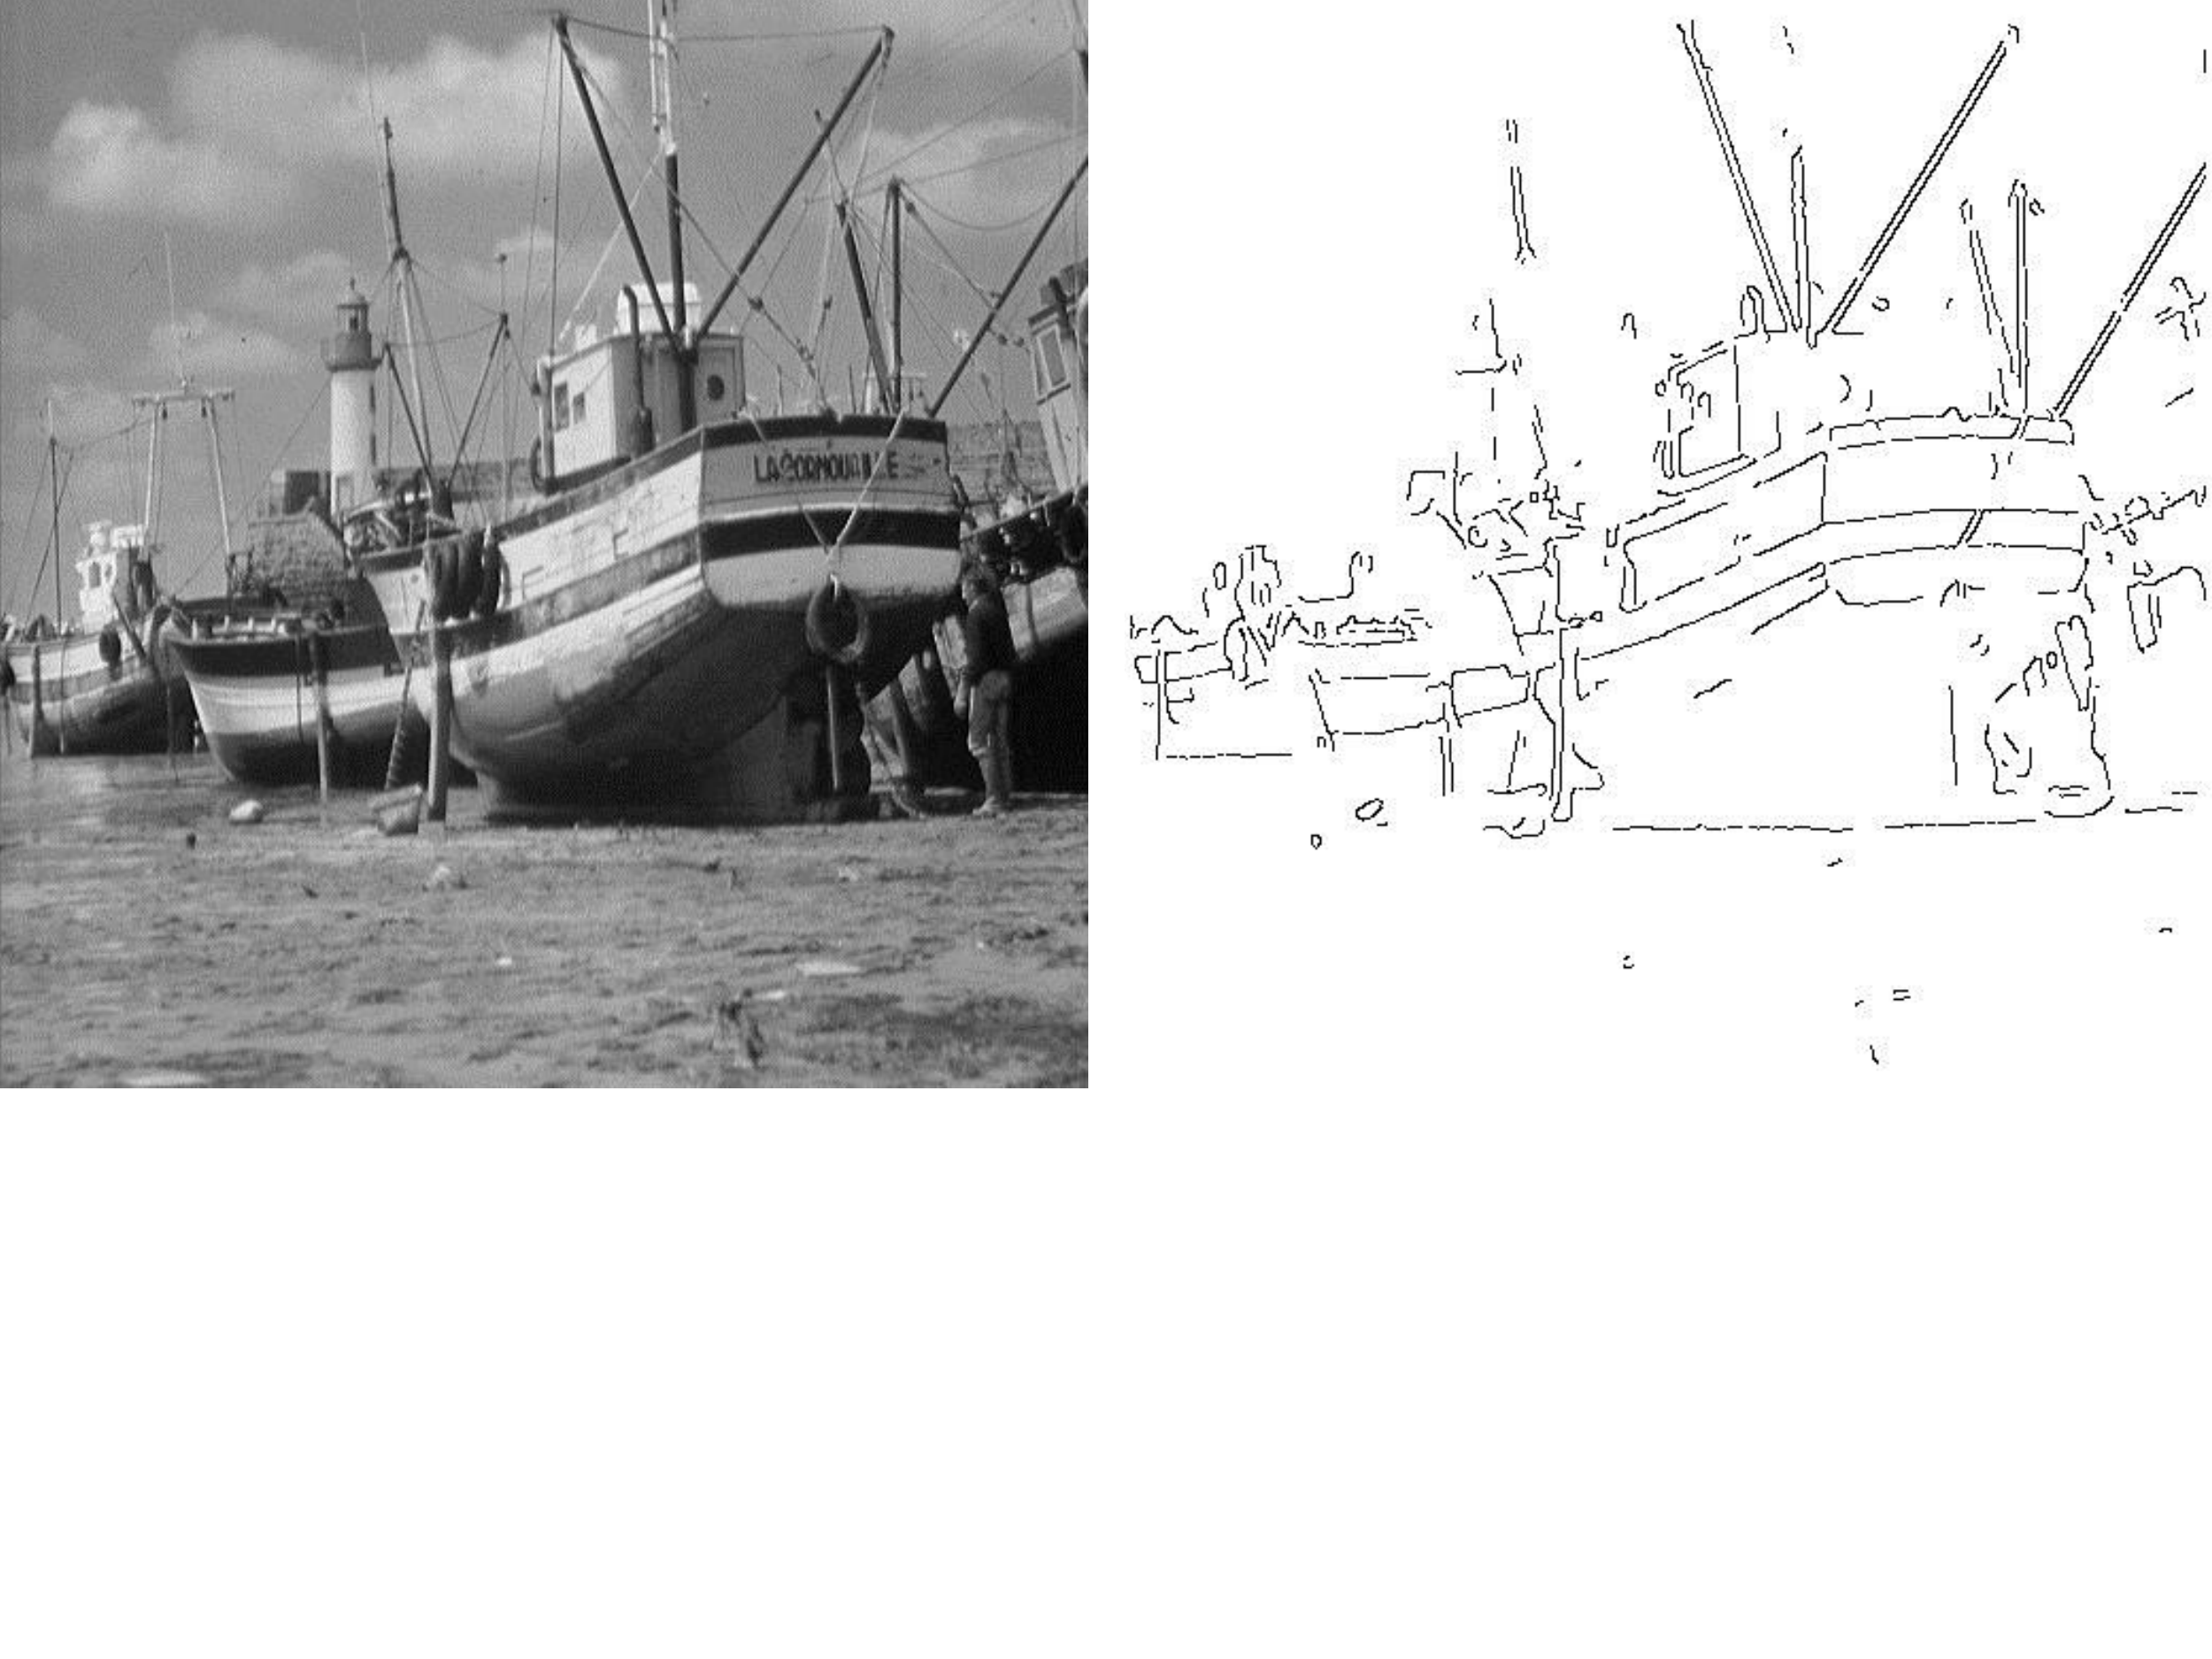}
    \caption{A boat image from USC-SIPI}
    \label{fig:dataset_dist}
    \vspace{-1ex} 
\end{figure}

\begin{figure}
    \centering
    \includegraphics[viewport=0 200 800 550, scale=0.32, clip=true]{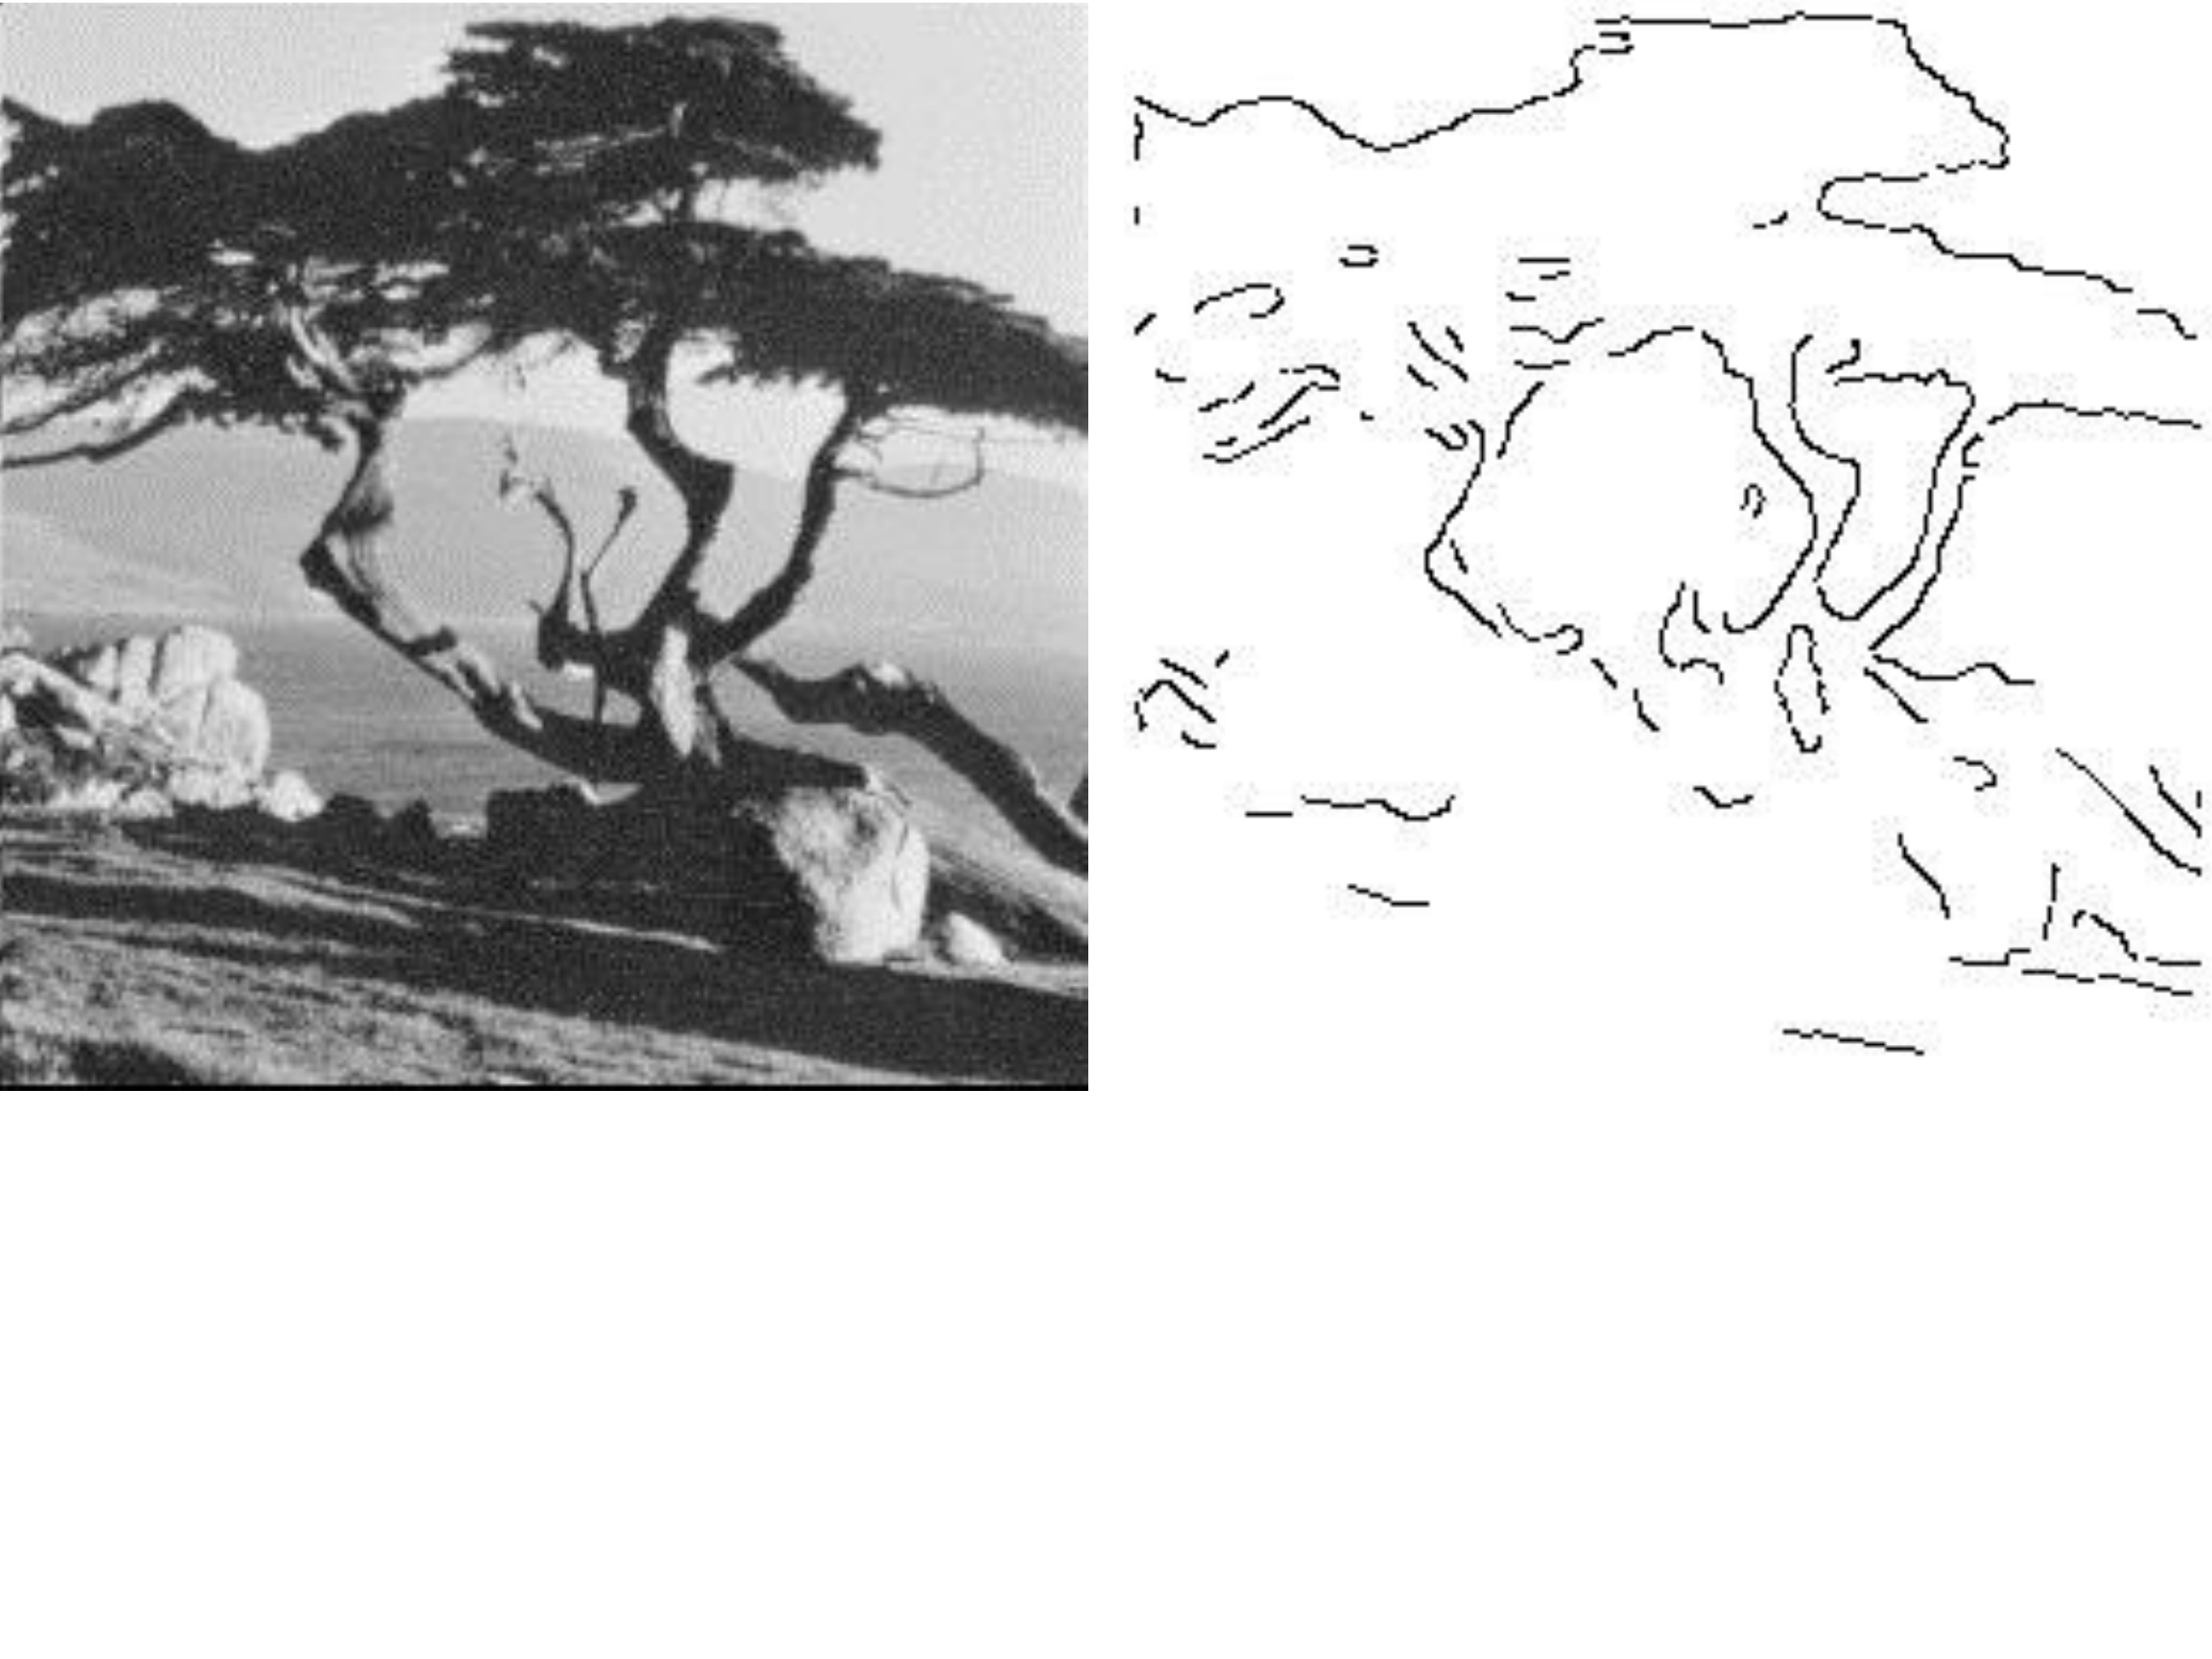}
    \caption{A tree from USC-SIPI}
    \label{fig:dataset_dist}
    \vspace{-1ex} 
\end{figure}

\begin{figure}
    \centering
    \includegraphics[viewport=0 200 800 550, scale=0.32, clip=true]{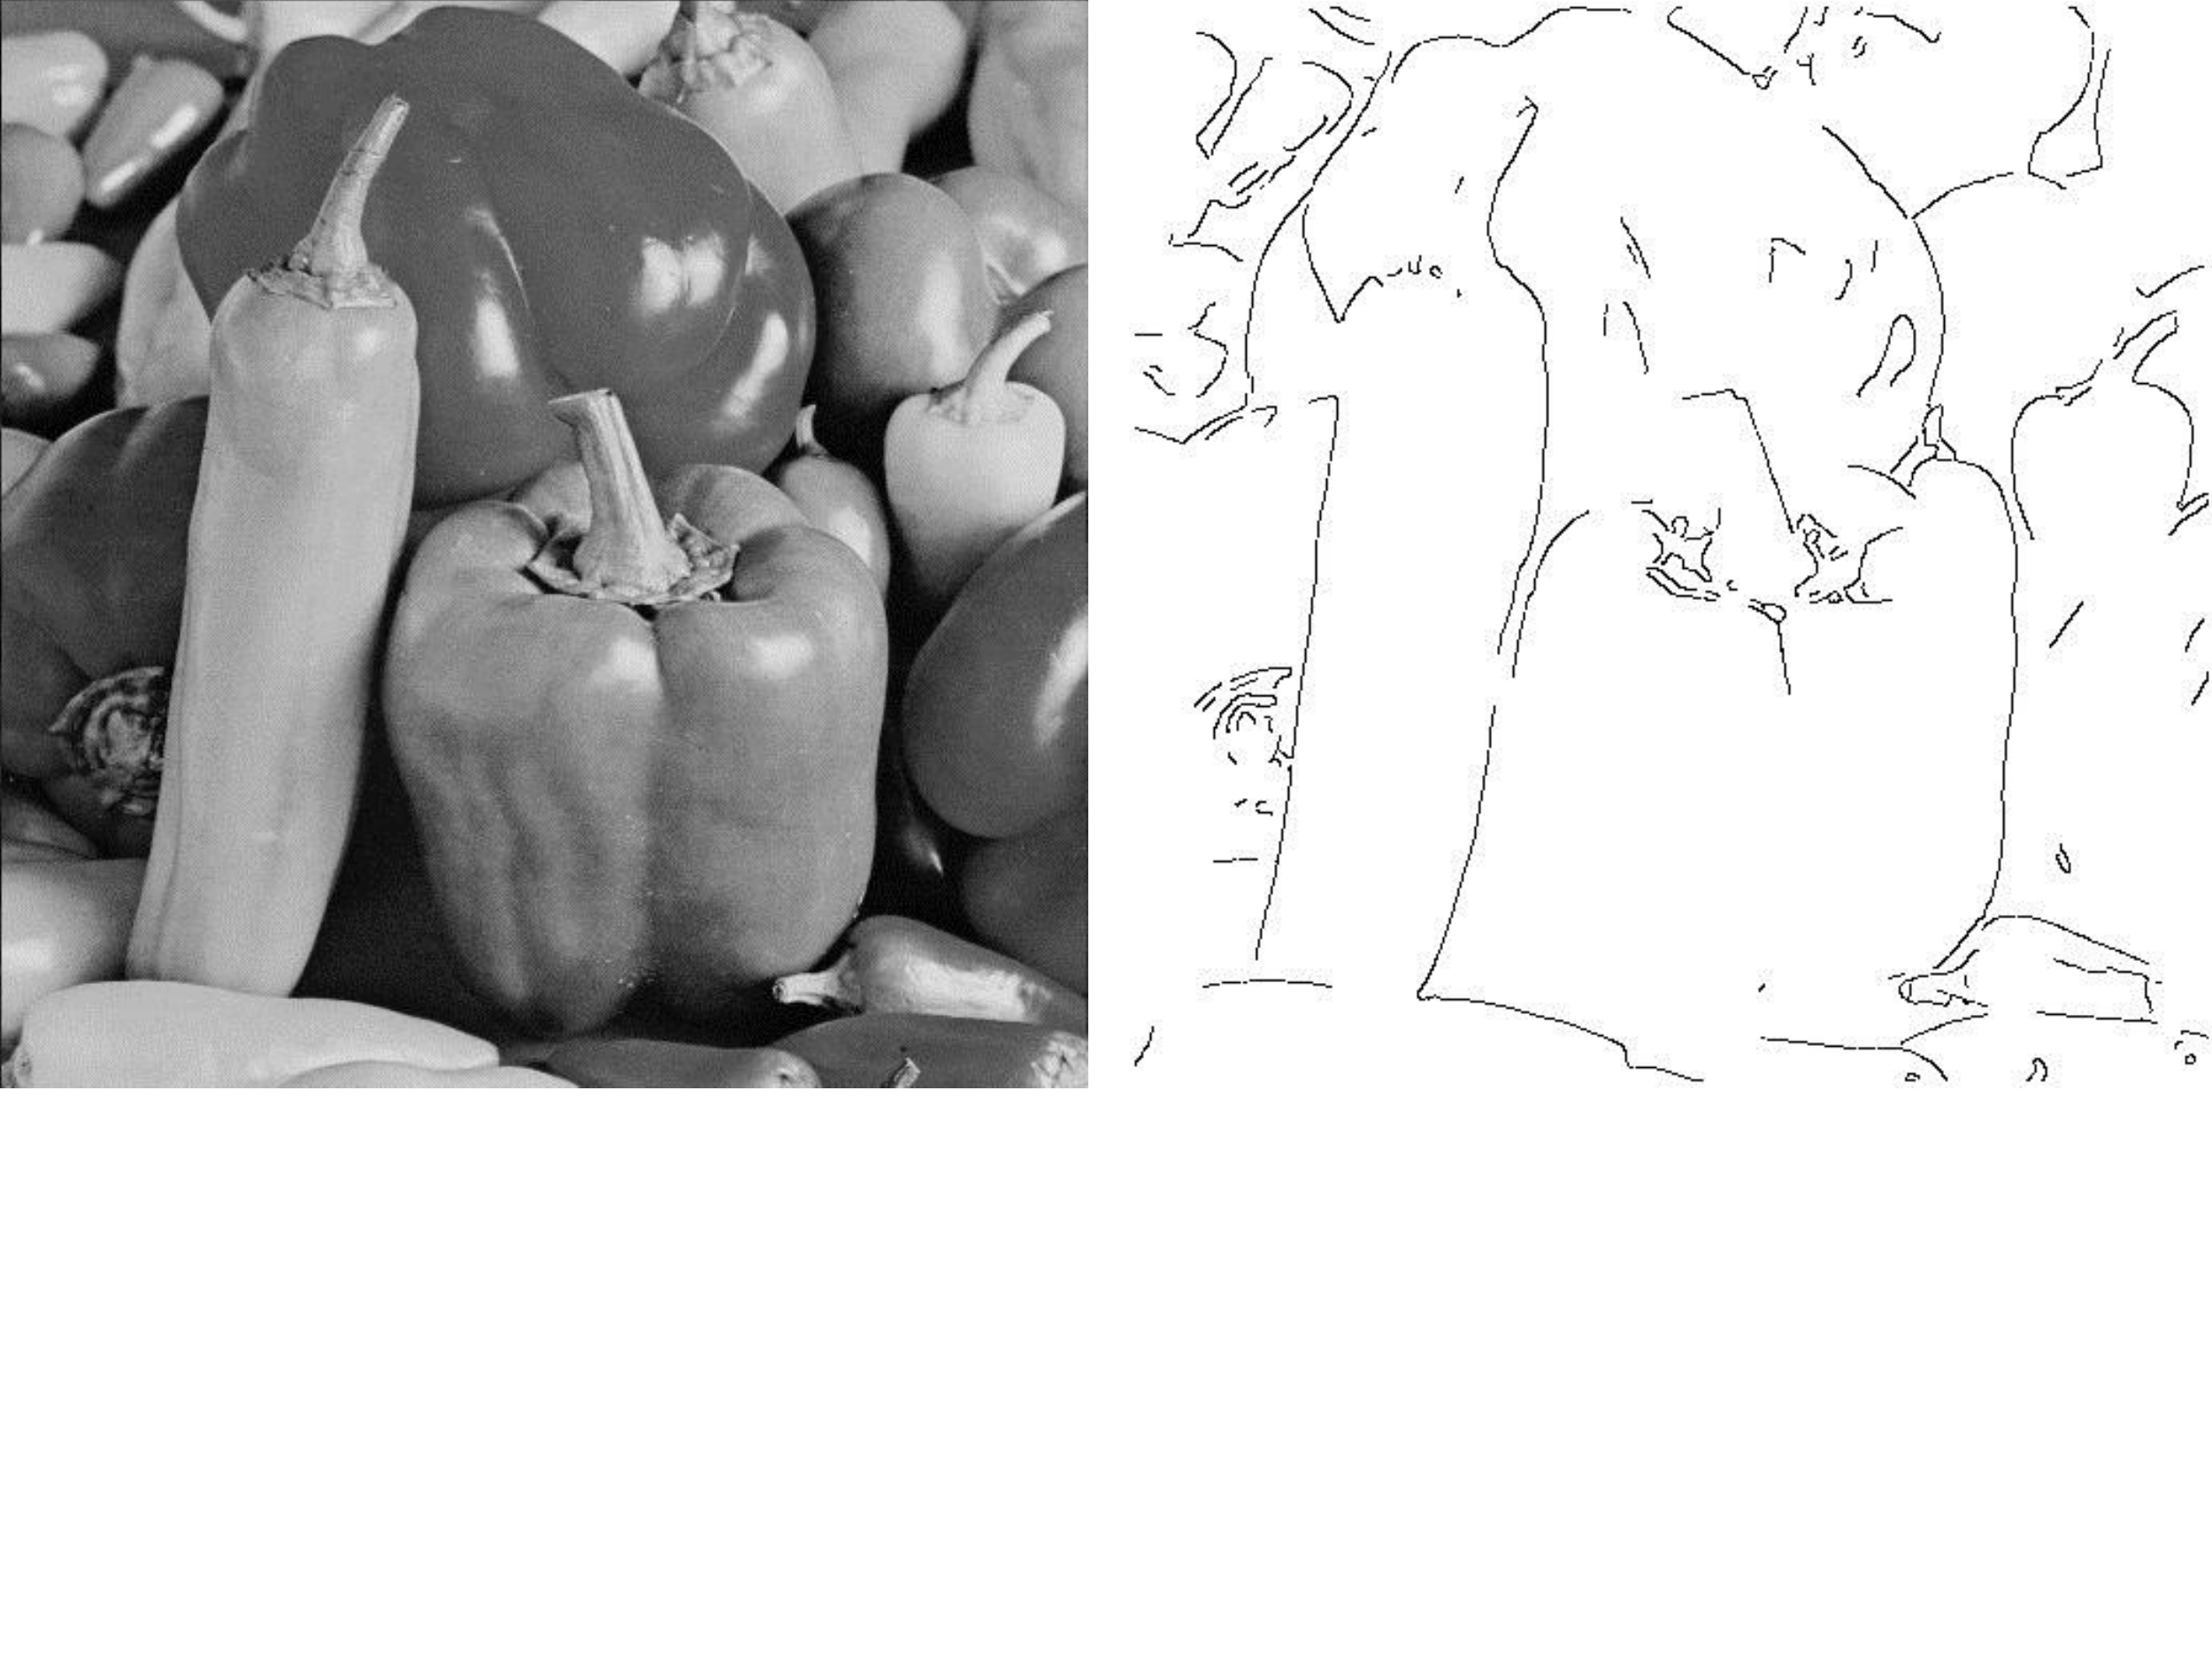}
    \caption{A vegitable image from USC-SIPI}
    \label{fig:dataset_dist}
    \vspace{-1ex} 
\end{figure}

\begin{figure}
    \centering
    \includegraphics[viewport=0 200 800 550, scale=0.32, clip=true]{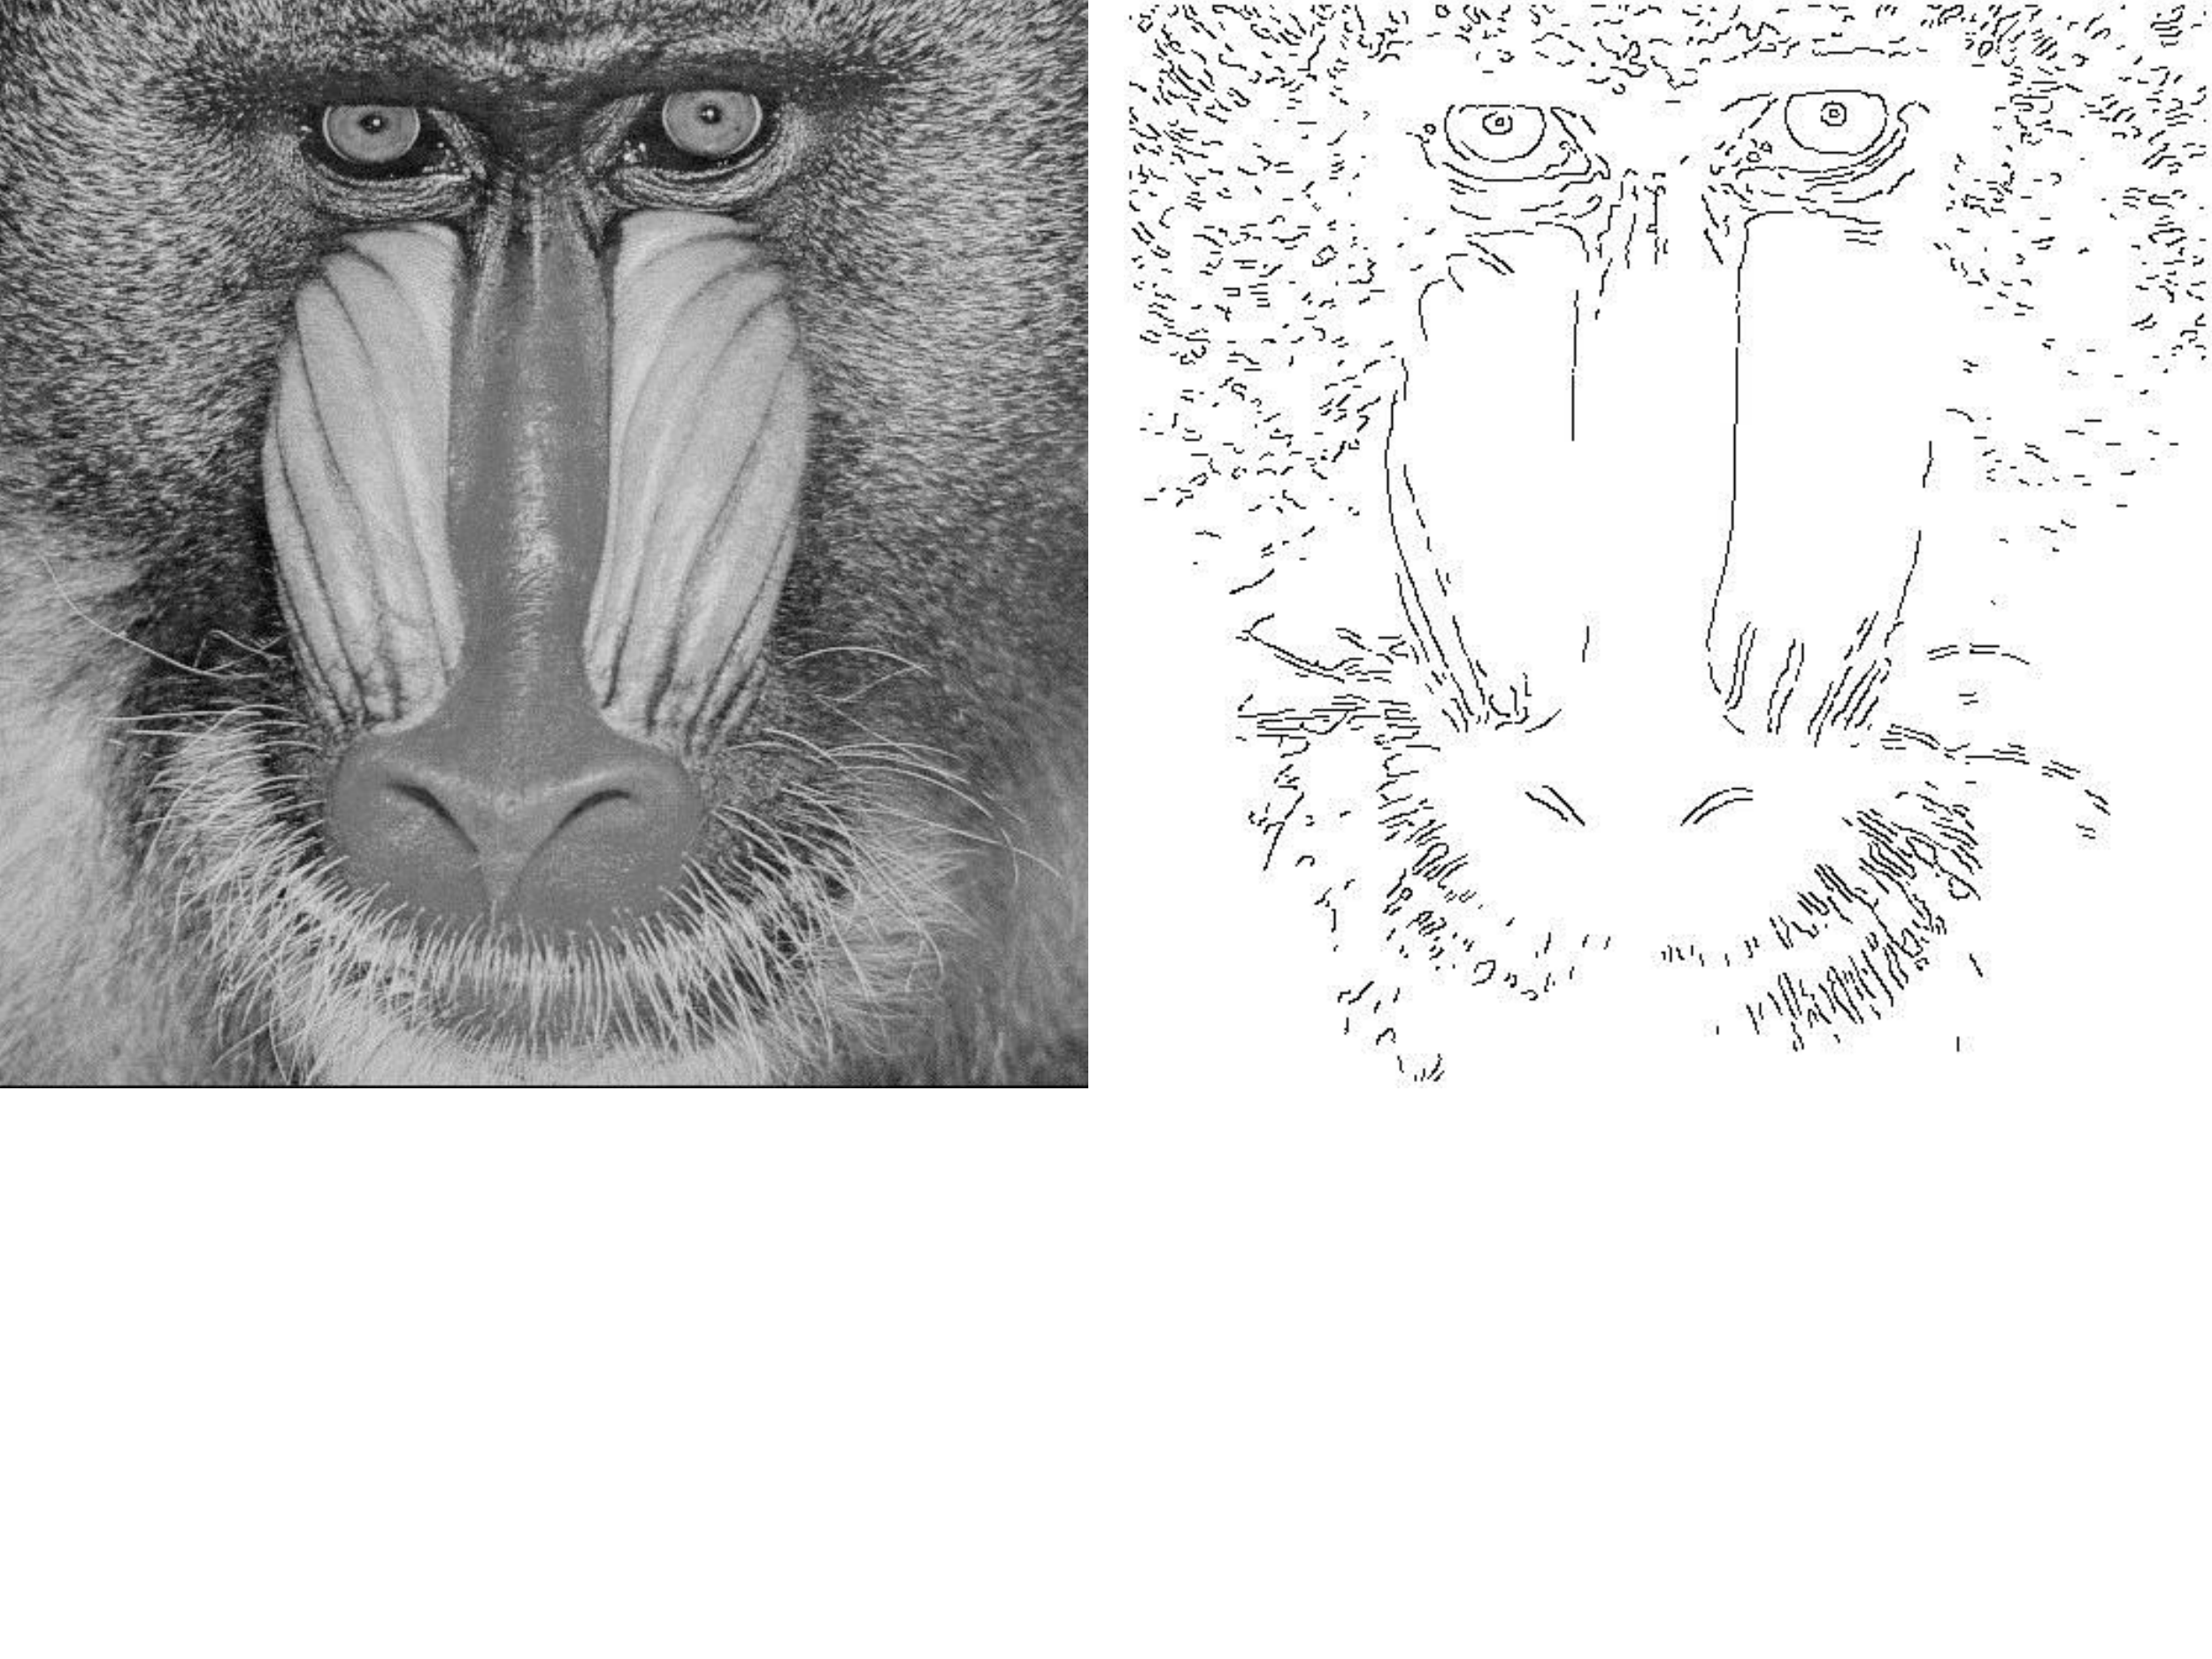}
    \caption{A baboon image from USC-SIPI}
    \label{fig:dataset_dist}
    \vspace{-1ex} 
\end{figure}
